# Supplementary material for: LICORICE: Label-Efficient Concept-Based Interpretable Reinforcement Learning
Source: arXiv:2407.15786 source file (2025-03-20)
Supplement: Supplementary file 1 [file 91-background-details.tex]

\section{Extended Background}

\subsection{Training Concept Bottleneck Models}
\label{sec:appx-training-cbm}
The CBM paper considers the following ways to learn a model $(\hat{f}, \hat{g})$:
\begin{enumerate}
    \item The \textit{independent bottleneck} learns $\hat{f}$ and $\hat{g}$ independently. Here, $$\hat{f} = \text{arg min}_f \sum_i L_Y(f(c^{(i)}); y^{(i)}) \text{ and} $$ $$\hat{g} = \text{arg min}_g \sum_{i,j} L_{C_j}(g_j(x^{(i)}); c_j^{(i)}).$$
    Note that $\hat{f}$ is trained using the true $c$, but at test time it takes $\hat{g}(x)$ as input.
    
    \item The \textit{sequential bottleneck} first learns $\hat{g}$ in the same way as above. 
    It then uses the concept predictions $\hat{g}(x)$ to learn $\hat{f} = \text{arg min}_f \sum_i L_Y(f(\hat{g}(x^{(i)})); y^{(i)}).$
    \item The \textit{joint bottleneck} minimizes the weighted sum
    \[
        \hat{f}, \hat{g} = \text{arg min}_{f,g} \sum_i \left[ L_Y(f(g(x^{(i)})); y^{(i)}) + \sum_j \lambda L_C(g(x^{(i)}); c^{(i)}) \right]
    \]
    for some $\lambda > 0$.    
    \item Finally, the \textit{standard model} ignores concepts and directly minimizes $\hat{f}, \hat{g} = \text{arg min}_{f,g} \sum_i L_Y(f(g(x^{(i)})); y^{(i)})$.
\end{enumerate}

The hyperparameter $\lambda$ in the joint bottleneck controls the tradeoff between concept vs. task loss. The standard model is equivalent to taking $\lambda \rightarrow 0$, while the sequential bottleneck can be viewed as taking $\lambda \rightarrow \infty$.
Interestingly, it seems like all techniques perform similarly well in the original paper.
